# Supplementary material for: Superconductivity-induced improper orders
Source: arXiv:2309.05664 ancillary file (2023-09-11)
Supplement: Supplementary file 1 [file SupplementalInformation.pdf]

# Supplemental Information
# Superconductivity-induced improper orders

András L. Szabó
*Institute for Theoretical Physics, ETH Zurich, 8093 Zurich, Switzerland*

Aline Ramires
*Paul Scherrer Institute, 5232 Villigen PSI, Switzerland*

(Dated: September 11, 2023)

## I. EXTENSION OF SPACE GROUP P4/nmm

Here we discuss in detail the two unit-cell extension of the nonsymmorphic space group P4/nmm (# 129) and the emergence of new types of double-valued irreducible representations (irreps). We start defining the operations and their multiplication table. From the multiplication table, we can deduce the conjugacy classes and the character table. We begin analyzing P4/nmm module integer lattice vector translations, corresponding to what we call the one unit-cell scenario. We use these structures as the basis to discuss the extended version of the group, which we call the two unit-cell scenario.

### A. Introducing space group P4/nmm

P4/nmm consists of 16 symmetry operations. Below, we label all the operations in three different ways: i) numerical label by $O_{i=1,\ldots,16}$; ii) concise label, by taking the associated point group operation (an extra bar indicates the operations that are accompanied by a single half primitive lattice vector (PLV) translation, while a tilde indicates the operation is accompanied by two orthogonal half PLV translations; and iii) standard Seitz label. We also provide the result of the space group operations on the Cartesian coordinates (x,y,z). The PLVs used here are $\mathbf{t_x} = (a, 0, 0)$ and $\mathbf{t_y} = (0, a, 0)$, where $a$ is the in-plane unit cell dimension, which we take to be equal to one in the following.

$$
\begin{aligned}
O_1 :&\quad E \equiv \{E|\mathbf{0}\} : (x, y, z) \qquad (1)\\
O_2 :&\quad \tilde{C}_{2z} \equiv \{C_{2z}|\mathbf{t_x}/2 + \mathbf{t_y}/2\} : (1/2 - x, 1/2 - y, z)\\
O_3 :&\quad \bar{C}_{4z} \equiv \{C_{4z}|\mathbf{t_x}/2\} : (1/2 - y, x, z)\\
O_4 :&\quad \bar{C}^{-1}_{4z} \equiv \{C^{-1}_{4z}|\mathbf{t_y}/2\} : (y, 1/2 - x, z)\\
O_5 :&\quad \bar{\sigma}_x \equiv \{\sigma_x|\mathbf{t_x}/2\} : (1/2 - x, y, z)\\
O_6 :&\quad \bar{\sigma}_y \equiv \{\sigma_y|\mathbf{t_y}/2\} : (x, 1/2 - y, z)\\
O_7 :&\quad \sigma_d \equiv \{\sigma_d|\mathbf{0}\} : (y, x, z)\\
O_8 :&\quad \tilde{\sigma}_{\bar{d}} \equiv \{\sigma_{\bar{d}}|\mathbf{t_x}/2 + \mathbf{t_y}/2\} : (1/2 - y, 1/2 - x, z)\\
O_9 :&\quad i \equiv \{i|\mathbf{0}\} : (-x, -y, -z)\\
O_{10} :&\quad \tilde{\sigma}_h \equiv \{\sigma_h|\mathbf{t_x}/2 + \mathbf{t_y}/2\} : (1/2 + x, 1/2 + y, -z)\\
O_{11} :&\quad \bar{S}_4 \equiv \{S_4|\mathbf{t_x}/2\} : (1/2 + y, -x, -z)\\
O_{12} :&\quad \bar{S}^{-1}_4 \equiv \{S^{-1}_4|\mathbf{t_y}/2\} : (-y, 1/2 + x, -z)\\
O_{13} :&\quad \bar{C}_{2y} \equiv \{C_{2y}|\mathbf{t_x}/2\} : (1/2 + x, -y, -z)\\
O_{14} :&\quad \bar{C}_{2x} \equiv \{C_{2x}|\mathbf{t_y}/2\} : (-x, 1/2 + y, -z)\\
O_{15} :&\quad C_{2\bar{d}} \equiv \{C_{2\bar{d}}|\mathbf{0}\} : (-y, -x, -z)\\
O_{16} :&\quad \tilde{C}_{2d} \equiv \{C_{2d}|\mathbf{t_x}/2 + \mathbf{t_y}/2\} : (1/2 + y, 1/2 + x, -z)
\end{aligned}
$$

### B. Irreducible representations for the single unit-cell scenario

Following the definition of the 16 operators listed in Eq. 1 above, we can construct the multiplication table modulo integer lattice translations. The result is displayed as Table I, and corresponds to the little group at the $\Gamma$ point. This group is isomorphic to the abstract group $G^9_{16}$ [1].

TABLE I. Multiplication table for elements in the space group P4/nmm modulo integer lattice translations. Here we use the numerical notation $O_{i=1,\ldots,16}$.

| | $\mathbf{O_1}$ | $\mathbf{O_2}$ | $\mathbf{O_3}$ | $\mathbf{O_4}$ | $\mathbf{O_5}$ | $\mathbf{O_6}$ | $\mathbf{O_7}$ | $\mathbf{O_8}$ | $\mathbf{O_9}$ | $\mathbf{O_{10}}$ | $\mathbf{O_{11}}$ | $\mathbf{O_{12}}$ | $\mathbf{O_{13}}$ | $\mathbf{O_{14}}$ | $\mathbf{O_{15}}$ | $\mathbf{O_{16}}$ |
|---|---|---|---|---|---|---|---|---|---|---|---|---|---|---|---|---|
| $\mathbf{O_1}$ | $O_1$ | $O_2$ | $O_3$ | $O_4$ | $O_5$ | $O_6$ | $O_7$ | $O_8$ | $O_9$ | $O_{10}$ | $O_{11}$ | $O_{12}$ | $O_{13}$ | $O_{14}$ | $O_{15}$ | $O_{16}$ |
| $\mathbf{O_2}$ | $O_2$ | $O_1$ | $O_4$ | $O_3$ | $O_6$ | $O_5$ | $O_8$ | $O_7$ | $O_{10}$ | $O_9$ | $O_{12}$ | $O_{11}$ | $O_{14}$ | $O_{13}$ | $O_{16}$ | $O_{15}$ |
| $\mathbf{O_3}$ | $O_3$ | $O_4$ | $O_2$ | $O_1$ | $O_7$ | $O_8$ | $O_6$ | $O_5$ | $O_{11}$ | $O_{12}$ | $O_{10}$ | $O_9$ | $O_{15}$ | $O_{16}$ | $O_{14}$ | $O_{13}$ |
| $\mathbf{O_4}$ | $O_4$ | $O_3$ | $O_1$ | $O_2$ | $O_8$ | $O_7$ | $O_5$ | $O_6$ | $O_{12}$ | $O_{11}$ | $O_9$ | $O_{10}$ | $O_{16}$ | $O_{15}$ | $O_{13}$ | $O_{14}$ |
| $\mathbf{O_5}$ | $O_5$ | $O_6$ | $O_8$ | $O_7$ | $O_1$ | $O_2$ | $O_4$ | $O_3$ | $O_{13}$ | $O_{14}$ | $O_{16}$ | $O_{15}$ | $O_9$ | $O_{10}$ | $O_{12}$ | $O_{11}$ |
| $\mathbf{O_6}$ | $O_6$ | $O_5$ | $O_7$ | $O_8$ | $O_2$ | $O_1$ | $O_3$ | $O_4$ | $O_{14}$ | $O_{13}$ | $O_{15}$ | $O_{16}$ | $O_{10}$ | $O_9$ | $O_{11}$ | $O_{12}$ |
| $\mathbf{O_7}$ | $O_7$ | $O_8$ | $O_5$ | $O_6$ | $O_3$ | $O_4$ | $O_1$ | $O_2$ | $O_{15}$ | $O_{16}$ | $O_{13}$ | $O_{14}$ | $O_{11}$ | $O_{12}$ | $O_9$ | $O_{10}$ |
| $\mathbf{O_8}$ | $O_8$ | $O_7$ | $O_6$ | $O_5$ | $O_4$ | $O_3$ | $O_2$ | $O_1$ | $O_{16}$ | $O_{15}$ | $O_{14}$ | $O_{13}$ | $O_{12}$ | $O_{11}$ | $O_{10}$ | $O_9$ |
| $\mathbf{O_9}$ | $O_9$ | $O_{10}$ | $O_{11}$ | $O_{12}$ | $O_{13}$ | $O_{14}$ | $O_{15}$ | $O_{16}$ | $O_1$ | $O_2$ | $O_3$ | $O_4$ | $O_5$ | $O_6$ | $O_7$ | $O_8$ |
| $\mathbf{O_{10}}$ | $O_{10}$ | $O_9$ | $O_{12}$ | $O_{11}$ | $O_{14}$ | $O_{13}$ | $O_{16}$ | $O_{15}$ | $O_2$ | $O_1$ | $O_4$ | $O_3$ | $O_6$ | $O_5$ | $O_8$ | $O_7$ |
| $\mathbf{O_{11}}$ | $O_{11}$ | $O_{12}$ | $O_{10}$ | $O_9$ | $O_{15}$ | $O_{16}$ | $O_{14}$ | $O_{13}$ | $O_3$ | $O_4$ | $O_2$ | $O_1$ | $O_7$ | $O_8$ | $O_6$ | $O_5$ |
| $\mathbf{O_{12}}$ | $O_{12}$ | $O_{11}$ | $O_9$ | $O_{10}$ | $O_{16}$ | $O_{15}$ | $O_{13}$ | $O_{14}$ | $O_4$ | $O_3$ | $O_1$ | $O_2$ | $O_8$ | $O_7$ | $O_5$ | $O_6$ |
| $\mathbf{O_{13}}$ | $O_{13}$ | $O_{14}$ | $O_{16}$ | $O_{15}$ | $O_9$ | $O_{10}$ | $O_{12}$ | $O_{11}$ | $O_5$ | $O_6$ | $O_8$ | $O_7$ | $O_1$ | $O_2$ | $O_4$ | $O_3$ |
| $\mathbf{O_{14}}$ | $O_{14}$ | $O_{13}$ | $O_{15}$ | $O_{16}$ | $O_{10}$ | $O_9$ | $O_{11}$ | $O_{12}$ | $O_6$ | $O_5$ | $O_7$ | $O_8$ | $O_2$ | $O_1$ | $O_3$ | $O_4$ |
| $\mathbf{O_{15}}$ | $O_{15}$ | $O_{16}$ | $O_{13}$ | $O_{14}$ | $O_{11}$ | $O_{12}$ | $O_9$ | $O_{10}$ | $O_7$ | $O_8$ | $O_5$ | $O_6$ | $O_3$ | $O_4$ | $O_1$ | $O_2$ |
| $\mathbf{O_{16}}$ | $O_{16}$ | $O_{15}$ | $O_{14}$ | $O_{13}$ | $O_{12}$ | $O_{11}$ | $O_{10}$ | $O_9$ | $O_8$ | $O_7$ | $O_6$ | $O_5$ | $O_4$ | $O_3$ | $O_2$ | $O_1$ |

The conjugacy classes can be obtained by checking which elements are conjugate to each other. The conjugation of operation $O_B$ by operation $O_A$ corresponds to $O_A.O_B.O_A^{-1} = O_C$, where the dot stands for the composition of operations. If $O_C \neq O_B$, this identity indicates that $O_B$ and $O_C$ belong to the same class. By inspection, we find 10 conjugacy classes:

$$
\begin{aligned}
&C_1 = \{O_1\}, && C_6 = \{O_9\}, \\
&C_2 = \{O_2\}, && C_7 = \{O_{10}\}, \\
&C_3 = \{O_3, O_4\}, && C_8 = \{O_{11}, O_{12}\}, \\
&C_4 = \{O_5, O_6\}, && C_9 = \{O_{13}, O_{14}\}, \\
&C_5 = \{O_7, O_8\}, && C_{10} = \{O_{15}, O_{16}\}.
\end{aligned}
\tag{2}
$$

From elementary group theory theorems, we know that the number of irreducible representations (irreps) equals the number of conjugacy classes [1]. The irreducible representations are associated with an array of characters (traces of the matrix representation of the corresponding operations in a given class), what constitutes the character table. Character tables can be derived based on fundamental properties of the irreducible representations but can also be found in the literature. For the case at hand, we find that P4/nmm modulo integer lattice translations is the little group at the $\Gamma$ point, which is isomorphic to the abstract group $G^9_{16}$ [1]. The corresponding character table is reproduced in Table II.

| | $E$ | $\tilde{C}_{2z}$ | $2\bar{C}_{4z}$ | $2\bar{\sigma}_x$ | $2\sigma_d$ | $i$ | $\tilde{\sigma}_h$ | $2\bar{S}_4$ | $2\bar{C}_{2x}$ | $2C_{2\bar{d}}$ |
|---|---|---|---|---|---|---|---|---|---|---|
| $A_{1g}$ | 1 | 1 | 1 | 1 | 1 | 1 | 1 | 1 | 1 | 1 |
| $A_{2g}$ | 1 | 1 | 1 | -1 | -1 | 1 | 1 | 1 | -1 | -1 |
| $B_{1g}$ | 1 | 1 | -1 | 1 | -1 | 1 | 1 | -1 | 1 | -1 |
| $B_{2g}$ | 1 | 1 | -1 | -1 | 1 | 1 | 1 | -1 | -1 | 1 |
| $E_g$ | 2 | -2 | 0 | 0 | 0 | 2 | -2 | 0 | 0 | 0 |
| $A_{1u}$ | 1 | 1 | 1 | -1 | -1 | -1 | -1 | -1 | 1 | 1 |
| $A_{2u}$ | 1 | 1 | 1 | 1 | 1 | -1 | -1 | -1 | -1 | -1 |
| $B_{1u}$ | 1 | 1 | -1 | -1 | 1 | -1 | -1 | 1 | 1 | -1 |
| $B_{2u}$ | 1 | 1 | -1 | 1 | -1 | -1 | -1 | 1 | -1 | 1 |
| $E_u$ | 2 | -2 | 0 | 0 | 0 | -2 | 2 | 0 | 0 | 0 |

TABLE II. Character table for the 10 irreps in the space group P4/nmm modulo primitive lattice vector translations, corresponding to the single unit cell scenario. The irreps listed in the first column are labelled according to the standard Mullikan notation. The conjugacy classes listed in the first row are labelled by a representative element (in the concise notation) preceded by the number of elements in the class.

### C. Introducing the extended space group P4/nmm

Once we double the unit cell (see Fig. 2 in the main text), we introduce new non-trivial symmetry elements associated with an extra PLV translation, which we here choose to be $O_{17} : E' \equiv \{E|\mathbf{t_y}\}$. Following the notation above, we label all the operations in three different ways: i) numerical label by $O_{i=1,\ldots,32}$, with $O_{i+16} = O_{17}.O_i$; ii) concise label, by taking the associated point group operation (now a prime corresponds to the extended operation); and iii) standard Seitz label. We again provide the result of the space group operations on the Cartesian coordinates (x,y,z). Note that the operations $O_{1,\ldots,16}$ are the same as above, so here we list only the extended operations $O_{17,\ldots32}$.

$$
\begin{aligned}
&O_{17}: \ E' \equiv \{E|\mathbf{t_y}\} : (x, y+1, z) \\
&O_{18}: \ \tilde{C}'_{2z} \equiv \{C_{2z}|\mathbf{t_x}/2 + 3\mathbf{t_y}/2\} : (1/2 - x, 3/2 - y, z) \\
&O_{19}: \ \bar{C}'_{4z} \equiv \{C_{4z}|\mathbf{t_x}/2 + \mathbf{t_y}\} : (1/2 - y, x+1, z) \\
&O_{20}: \ \bar{C}^{-1\prime}_{4z} \equiv \{C^{-1}_{4z}|3\mathbf{t_y}/2\} : (y, 3/2 - x, z) \\
&O_{21}: \ \bar{\sigma}'_x \equiv \{\sigma_x|\mathbf{t_x}/2 + \mathbf{t_y}\} : (1/2 - x, y+1, z) \\
&O_{22}: \ \bar{\sigma}'_y \equiv \{\sigma_y|3\mathbf{t_y}/2\} : (x, 3/2 - y, z) \\
&O_{23}: \ \sigma'_d \equiv \{\sigma_d|\mathbf{t_y}\} : (y, x+1, z) \\
&O_{24}: \ \tilde{\sigma}'_{\bar{d}} \equiv \{\sigma_{\bar{d}}|\mathbf{t_x}/2 + 3\mathbf{t_y}/2\} : (1/2 - y, 3/2 - x, z) \\
&O_{25}: \ i' \equiv \{i|\mathbf{t_y}\} : (-x, -y+1, -z) \\
&O_{26}: \ \tilde{\sigma}'_h \equiv \{\sigma_h|\mathbf{t_x}/2 + 3\mathbf{t_y}/2\} : (1/2 + x, 3/2 + y, -z) \\
&O_{27}: \ \bar{S}'_4 \equiv \{S_4|\mathbf{t_x}/2 + \mathbf{t_y}\} : (1/2 + y, -x+1, -z) \\
&O_{28}: \ \bar{S}'^{-1}_4 \equiv \{S^{-1}_4|3\mathbf{t_y}/2\} : (-y, 3/2 + x, -z) \\
&O_{29}: \ \bar{C}'_{2y} \equiv \{C_{2y}|\mathbf{t_x}/2 + \mathbf{t_y}\} : (1/2 + x, -y+1, -z) \\
&O_{30}: \ \bar{C}'_{2x} \equiv \{C_{2x}|3\mathbf{t_y}/2\} : (-x, 3/2 + y, -z) \\
&O_{31}: \ C'_{2\bar{d}} \equiv \{C_{2\bar{d}}|\mathbf{t_y}\} : (-y, -x+1, -z) \\
&O_{32}: \ \tilde{C}'_{2d} \equiv \{C_{2d}|\mathbf{t_x}/2 + 3\mathbf{t_y}/2\} : (1/2 + y, 3/2 + x, -z)
\end{aligned}
\tag{3}
$$

### D. Irreducible representations for the doubled unit-cell scenario

The product table for the group formed by the 32 operations introduced above modulo two basis vector translations is displayed as Table III.

TABLE III. Multiplication table for elements in the space group P4/nmm modulo two integer lattice translations. Here we use the numerical notation $O_{i=1,\ldots,32}$. The remaining products are obtained by the following rules: i) $O_{i+16}.O_{j+16} = O_i.O_j$, ii) If $O_i.O_j = O_k$, then $O_{i+16}.O_j = O_{mod(k+16,32)}$, and $O_i.O_{j+16} = O_{mod(k+16,32)}$.

| | $\mathbf{O_1}$ | $\mathbf{O_2}$ | $\mathbf{O_3}$ | $\mathbf{O_4}$ | $\mathbf{O_5}$ | $\mathbf{O_6}$ | $\mathbf{O_7}$ | $\mathbf{O_8}$ | $\mathbf{O_9}$ | $\mathbf{O_{10}}$ | $\mathbf{O_{11}}$ | $\mathbf{O_{12}}$ | $\mathbf{O_{13}}$ | $\mathbf{O_{14}}$ | $\mathbf{O_{15}}$ | $\mathbf{O_{16}}$ |
|---|---|---|---|---|---|---|---|---|---|---|---|---|---|---|---|---|
| $\mathbf{O_1}$ | $O_1$ | $O_2$ | $O_3$ | $O_4$ | $O_5$ | $O_6$ | $O_7$ | $O_8$ | $O_9$ | $O_{10}$ | $O_{11}$ | $O_{12}$ | $O_{13}$ | $O_{14}$ | $O_{15}$ | $O_{16}$ |
| $\mathbf{O_2}$ | $O_2$ | $O_1$ | $O_4$ | $O_3$ | $O_6$ | $O_5$ | $O_8$ | $O_7$ | $O_{10}$ | $O_9$ | $O_{12}$ | $O_{11}$ | $O_{14}$ | $O_{13}$ | $O_{16}$ | $O_{15}$ |
| $\mathbf{O_3}$ | $O_3$ | $O_4$ | $O_2$ | $O_1$ | $O_7$ | $O_8$ | $O_6$ | $O_5$ | $O_{27}$ | $O_{28}$ | $O_{26}$ | $O_{25}$ | $O_{31}$ | $O_{32}$ | $O_{30}$ | $O_{29}$ |
| $\mathbf{O_4}$ | $O_4$ | $O_3$ | $O_1$ | $O_2$ | $O_8$ | $O_7$ | $O_5$ | $O_6$ | $O_{28}$ | $O_{27}$ | $O_{25}$ | $O_{26}$ | $O_{32}$ | $O_{31}$ | $O_{29}$ | $O_{30}$ |
| $\mathbf{O_5}$ | $O_5$ | $O_6$ | $O_8$ | $O_7$ | $O_1$ | $O_2$ | $O_4$ | $O_3$ | $O_{29}$ | $O_{30}$ | $O_{32}$ | $O_{31}$ | $O_{25}$ | $O_{26}$ | $O_{28}$ | $O_{27}$ |
| $\mathbf{O_6}$ | $O_6$ | $O_5$ | $O_7$ | $O_8$ | $O_2$ | $O_1$ | $O_3$ | $O_4$ | $O_{30}$ | $O_{29}$ | $O_{31}$ | $O_{32}$ | $O_{26}$ | $O_{25}$ | $O_{27}$ | $O_{28}$ |
| $\mathbf{O_7}$ | $O_7$ | $O_8$ | $O_5$ | $O_6$ | $O_3$ | $O_4$ | $O_1$ | $O_2$ | $O_{15}$ | $O_{16}$ | $O_{13}$ | $O_{14}$ | $O_{11}$ | $O_{12}$ | $O_9$ | $O_{10}$ |
| $\mathbf{O_8}$ | $O_8$ | $O_7$ | $O_6$ | $O_5$ | $O_4$ | $O_3$ | $O_2$ | $O_1$ | $O_{16}$ | $O_{15}$ | $O_{14}$ | $O_{13}$ | $O_{12}$ | $O_{11}$ | $O_{10}$ | $O_9$ |
| $\mathbf{O_9}$ | $O_9$ | $O_{10}$ | $O_{11}$ | $O_{12}$ | $O_{13}$ | $O_{14}$ | $O_{15}$ | $O_{16}$ | $O_1$ | $O_2$ | $O_3$ | $O_4$ | $O_5$ | $O_6$ | $O_7$ | $O_8$ |
| $\mathbf{O_{10}}$ | $O_{10}$ | $O_9$ | $O_{12}$ | $O_{11}$ | $O_{14}$ | $O_{13}$ | $O_{16}$ | $O_{15}$ | $O_2$ | $O_1$ | $O_4$ | $O_3$ | $O_6$ | $O_5$ | $O_8$ | $O_7$ |
| $\mathbf{O_{11}}$ | $O_{11}$ | $O_{12}$ | $O_{10}$ | $O_9$ | $O_{15}$ | $O_{16}$ | $O_{14}$ | $O_{13}$ | $O_{19}$ | $O_{20}$ | $O_{18}$ | $O_{17}$ | $O_{23}$ | $O_{24}$ | $O_{22}$ | $O_{21}$ |
| $\mathbf{O_{12}}$ | $O_{12}$ | $O_{11}$ | $O_9$ | $O_{10}$ | $O_{16}$ | $O_{15}$ | $O_{13}$ | $O_{14}$ | $O_{20}$ | $O_{19}$ | $O_{17}$ | $O_{18}$ | $O_{24}$ | $O_{23}$ | $O_{21}$ | $O_{22}$ |
| $\mathbf{O_{13}}$ | $O_{13}$ | $O_{14}$ | $O_{16}$ | $O_{15}$ | $O_9$ | $O_{10}$ | $O_{12}$ | $O_{11}$ | $O_{21}$ | $O_{22}$ | $O_{24}$ | $O_{23}$ | $O_{17}$ | $O_{18}$ | $O_{20}$ | $O_{19}$ |
| $\mathbf{O_{14}}$ | $O_{14}$ | $O_{13}$ | $O_{15}$ | $O_{16}$ | $O_{10}$ | $O_9$ | $O_{11}$ | $O_{12}$ | $O_{22}$ | $O_{21}$ | $O_{23}$ | $O_{24}$ | $O_{18}$ | $O_{17}$ | $O_{19}$ | $O_{20}$ |
| $\mathbf{O_{15}}$ | $O_{15}$ | $O_{16}$ | $O_{13}$ | $O_{14}$ | $O_{11}$ | $O_{12}$ | $O_9$ | $O_{10}$ | $O_7$ | $O_8$ | $O_5$ | $O_6$ | $O_3$ | $O_4$ | $O_1$ | $O_2$ |
| $\mathbf{O_{16}}$ | $O_{16}$ | $O_{15}$ | $O_{14}$ | $O_{13}$ | $O_{12}$ | $O_{11}$ | $O_{10}$ | $O_9$ | $O_8$ | $O_7$ | $O_6$ | $O_5$ | $O_4$ | $O_3$ | $O_2$ | $O_1$ |

Examining the conjugation relations, we find that there are 14 conjugacy classes, with elements organized as follows:

$$C_1 \to \begin{cases} C_1' = \{O_1\} \\ C_1'' = \{O_{17}\} \end{cases}$$

$$C_2 \to \begin{cases} C_2' = \{O_2\} \\ C_2'' = \{O_{18}\} \end{cases}$$

$$C_3 \to C_3' = \{O_3, O_4, O_{19}, O_{20}\}$$

$$C_4 \to C_4' = \{O_5, O_6, O_{21}, O_{22}\}$$

$$C_5 \to \begin{cases} C_5' = \{O_7, O_8\} \\ C_5'' = \{O_{23}, O_{24}\} \end{cases}$$

$$C_6 \to C_6' = \{O_9, O_{25}\}$$

$$C_7 \to C_7' = \{O_{10}, O_{26}\}$$

$$C_8 \to C_8' = \{O_{11}, O_{12}, O_{27}, O_{28}\}$$

$$C_9 \to C_9' = \{O_{13}, O_{14}, O_{29}, O_{30}\}$$

$$C_{10} = \to \begin{cases} C_{10}' = \{O_{15}, O_{32}\} \\ C_{10}'' = \{O_{16}, O_{31}\} \end{cases}$$

This extended group, with 32 elements organized in 14 conjugacy classes corresponds to the little group at the $M$ point, which is isomorphic to the abstract group $G_{32}^2$ [1]. The corresponding character table is reproduced in Table IV.

TABLE IV. Character table for the 14 irreps in the space group P4/nmm modulo two integer lattice translations, corresponding to the doubled unit cell scenario. The first ten irreps listed in the first column are labelled according to the irreps established for the single unit cell scenario above. Four new two-dimensional irreps are labelled as $E_{im}$, with $i = 1, ..., 4$, with the subscript $m$ corresponding to mixed parity. The conjugacy classes listed in the first row are labelled by a representative element (in the concise notation) preceded by the number of elements in the class.

| | $E$ | $E'$ | $\tilde{C}_{2z}$ | $\tilde{C}'_{2z}$ | $4\bar{C}_{4z}$ | $4\bar{\sigma}_x$ | $2\sigma_d$ | $2\sigma'_d$ | $2i$ | $2\tilde{\sigma}_h$ | $4\bar{S}_4$ | $4\bar{C}_{2x}$ | $2C_{2\bar{d}}$ | $2C'_{2\bar{d}}$ |
|---|---|---|---|---|---|---|---|---|---|---|---|---|---|---|
| $A_{1g}$ | 1 | 1 | 1 | 1 | 1 | 1 | 1 | 1 | 1 | 1 | 1 | 1 | 1 | 1 |
| $A_{2g}$ | 1 | 1 | 1 | 1 | 1 | -1 | -1 | -1 | 1 | 1 | 1 | -1 | -1 | -1 |
| $B_{1g}$ | 1 | 1 | 1 | 1 | -1 | 1 | -1 | -1 | 1 | 1 | -1 | 1 | -1 | -1 |
| $B_{2g}$ | 1 | 1 | 1 | 1 | -1 | -1 | 1 | 1 | 1 | 1 | -1 | -1 | 1 | 1 |
| $E_g$ | 2 | 2 | -2 | -2 | 0 | 0 | 0 | 0 | 2 | -2 | 0 | 0 | 0 | 0 |
| $A_{1u}$ | 1 | 1 | 1 | 1 | 1 | -1 | -1 | -1 | -1 | -1 | -1 | 1 | 1 | 1 |
| $A_{2u}$ | 1 | 1 | 1 | 1 | 1 | 1 | 1 | 1 | -1 | -1 | -1 | -1 | -1 | -1 |
| $B_{1u}$ | 1 | 1 | 1 | 1 | -1 | -1 | 1 | 1 | -1 | -1 | 1 | 1 | -1 | -1 |
| $B_{2u}$ | 1 | 1 | 1 | 1 | -1 | 1 | -1 | -1 | -1 | -1 | 1 | -1 | 1 | 1 |
| $E_u$ | 2 | 2 | -2 | -2 | 0 | 0 | 0 | 0 | -2 | 2 | 0 | 0 | 0 | 0 |
| $E_{1m}$ | 2 | -2 | 2 | -2 | 0 | 0 | 2 | -2 | 0 | 0 | 0 | 0 | 0 | 0 |
| $E_{2m}$ | 2 | -2 | 2 | -2 | 0 | 0 | -2 | 2 | 0 | 0 | 0 | 0 | 0 | 0 |
| $E_{3m}$ | 2 | -2 | -2 | 2 | 0 | 0 | 0 | 0 | 0 | 0 | 0 | 0 | 2 | -2 |
| $E_{4m}$ | 2 | -2 | -2 | 2 | 0 | 0 | 0 | 0 | 0 | 0 | 0 | 0 | -2 | 2 |

A few things are to be noted about the character table of the extended group. The conjugacy classes of the extended group correspond to either i) one larger conjugacy class, $C'_i$, encompassing elements in the conjugacy class $C_i$ in the single unit-cell scenario, plus new elements corresponding to the composition of these elements with $E'$; ii) two conjugacy classes, $C'_i$ and $C''_i$, each with the same number of elements as the conjugacy class $C_i$ in the single unit-cell scenario.

The characters for the (single-valued) irreps, the first ten lines in Table IV, correspond to the character of the irreps of the single unit-cell scenario with the same label, satisfying $\chi(C_i) = \chi(C'_i) = \chi(C''_i)$. For the (double-valued) irreps, the four last lines in Table IV, the characters associated with conjugacy classes that do not split under the extension are necessarily zero, as $\chi(C_i) = -\chi(C'_i)$ [1]. The last statement is true for classes $C'_3 \equiv 4\bar{C}_{4z}, C'_4 \equiv 4\bar{\sigma}_x, C'_6 \equiv 2i, C'_7 \equiv 2\sigma_h, C'_8 \equiv 4\bar{S}_4, C'_9 \equiv 4\bar{C}_{2x}$. The remaining characters can be determined using the orthonormality condition for characters [1].

Note that inversion symmetry in the extended group belongs to $C'_6 \equiv 2i$. This conjugacy class does not split under the group extension; therefore, the characters associated with the double-valued irreps are zero, and these two-dimensional irreps act on basis functions of opposite parity. By symmetry, these must be degenerate, so we have the unusual scenario of two degenerate order parameters with different parity in the two unit-cell scenario. This justifies the superscript "m" for the new irreps, corresponding to "mixed parity".

Before we conclude this section, we highlight the direct product relations between the irreps of the extended group.

$$
\begin{aligned}
A_{1u/g} \otimes A_{1u/g} &= A_{1g} \\
A_{2u/g} \otimes A_{2u/g} &= A_{1g} \\
B_{1u/g} \otimes B_{1u/g} &= A_{1g} \\
B_{2u/g} \otimes B_{2u/g} &= A_{1g} \\
E_{u/g} \otimes E_{u/g} &= A_{1g} \oplus A_{2g} \oplus B_{1g} \oplus B_{2g} \\
E_{1/2m} \otimes E_{1/2m} &= A_{1g} \oplus A_{2u} \oplus B_{2g} \oplus B_{1u} \\
E_{3/4m} \otimes E_{3/4m} &= A_{1g} \oplus A_{1u} \oplus B_{2u} \oplus B_{2g}
\end{aligned} \tag{4}
$$

Note that bilinears of order parameters associated with the one-dimensional irreps always belong to $A_{1g}$, the trivial irrep. Bilinears of order parameters associated with the two-dimensional irreps $E_{u/g}$ are always even parity. Bilinears of order parameters with $E_{1m}$ symmetry can have either even or odd parity.

## II. ORDER PARAMETER CLASSIFICATION FOR THE SINGLE UNIT CELL SCENARIO

We now use this extended group structure to highlight the unexpected coupling between superconductivity and magnetism in $CeRh_2As_2$. Within the primitive unit cell scenario, corresponding to homogenous phases, order parameters in the particle-particle and particle-hole sectors can be parametrized as

$$\Delta^{PP} = \sum_{a,b} d_{ab}^{PP} \hat{\tau}_a \otimes \hat{\sigma}_b, \qquad \Delta^{PH} = \sum_{a,b} d_{ab}^{PH} \hat{\tau}_a \otimes \hat{\sigma}_b (i\hat{\sigma}_2), \tag{5}$$

where $\hat{\tau}_i$ and $\hat{\sigma}_i$ are two-dimensional Pauli matrices $(i = 1, 2, 3)$ or the identity matrix $(i = 0)$ encoding the sublattice and spin degree of freedom, respectively. To assess the transformation properties of particle-particle order parameters, we consider the fermion bilinear $\Psi^\dagger \Delta^{PP} \Psi$. Here $\Psi$ is in real space and encompasses the internal degrees of freedom, It transforms as $\Psi \to U\Psi$ under some unitary symmetry transformation $U$. Accordingly, the order parameter matrix transforms as $\Delta^{PP} \to U \Delta^{PP} U^\dagger$. On the other hand, for particle-hole orders, the order parameter connects an electron with its time-reversed partner, which we incorporate with the help of the Nambu spinor written in real space as $\Psi_N = [\Psi, \Psi^*]^\intercal$. The matrix $\Delta^{PH}$ then occupies an off-diagonal element in this basis, and the corresponding bilinear is of the form $\Psi^\dagger \Delta^{PP} \Psi^*$. We can nevertheless examine the transformation properties of both particle-particle and particle-hole bilinears on equal footing by introducing a slightly modified Nambu basis $\tilde{\Psi}_N = [\Psi, \sigma_2 \Psi^*]^\intercal$, wherein we absorb the unitary part of the time reversal operator in the lower block $(\sigma_2)$. In this basis the particle-hole and particle-particle bilinears transform identically.

In the single unit cell scenario, the matrix operators of the generating transformations $i$, $\bar{C}_{4z}$, and $\sigma_d$ are of the form

$$M_{C_{4z}} = \tau_0 \otimes \frac{\sigma_0 - i\sigma_3}{\sqrt{2}}, \qquad M_i = \tau_1 \otimes \sigma_0, \qquad M_{\sigma_d} = \frac{i}{\sqrt{2}} \tau_0 \otimes (\sigma_1 - \sigma_2).$$

Based on the explicit form of the order parameters and symmetry transformations, we can uniquely classify the matrix-content of the order parameters according to the irreps shown in Table II.

| (sublattice, spin) | $i$ | $\bar{C}_{4z}$ | $\sigma_d$ | $C_{2\bar{d}}$ | $\mathcal{T}$ | irrep |
|---|---|---|---|---|---|---|
| (0,0) | + | + | + | + | + | $A_{1g}$ |
| (1,0) | + | + | + | + | + | $A_{1g}$ |
| (0,3) | + | + | − | − | − | $A_{2g}$ |
| (1,3) | + | + | − | − | − | $A_{2g}$ |
| {(0,1),(0,2)} | + | $i\sigma_2$ | $-\sigma_1$ | $-\sigma_1$ | − | $E_g$ |
| {(1,1),(1,2)} | + | $i\sigma_2$ | $-\sigma_1$ | $-\sigma_1$ | − | $E_g$ |
| (2,3) | − | + | − | + | + | $A_{1u}$ |
| (3,3) | − | + | − | + | − | $A_{1u}$ |
| (2,0) | − | + | + | − | − | $A_{2u}$ |
| (3,0) | − | + | + | − | + | $A_{2u}$ |
| {(2,1),(2,2)} | − | $i\sigma_2$ | $-\sigma_1$ | $\sigma_1$ | + | $E_u$ |
| {(3,1),(3,2)} | − | $i\sigma_2$ | $-\sigma_1$ | $\sigma_1$ | − | $E_u$ |

TABLE V. Classification of order parameters matrices in the single unit cell scenario. A pair of indices $(i,j)$ indicates the corresponding matrix $\tau_i \otimes \sigma_j$, as indicated in Eq. 5. Signs +/− indicate even/odd transformation under the given group operation, with $\mathcal{T}$ being time reversal (applicable only to PP orders). For two-component order parameters, the transformations are realized by the given Pauli matrix acting on the appropriate two-dimensional basis functions. All other notation is identical to the main text. Blue and gray correspond to the $M_z$ antiferromagnetic and $P_z$ polar orders, respectively.

## III. ORDER PARAMETER CLASSIFICATION FOR THE DOUBLED UNIT CELL

We now use the extended group structure to classify all order parameters in the particle-particle and particle-hole sectors. These can be parametrized as

$$\Delta^{PP} = \sum_{a,b,c} d^{PP}_{abc} \hat{\eta}_a \otimes \hat{\tau}_b \otimes \hat{\sigma}_c, \qquad \Delta^{PH} = \sum_{a,b,c} d^{PH}_{abc} \hat{\eta}_a \otimes \hat{\tau}_b \otimes \hat{\sigma}_c (i\hat{\sigma}_2), \tag{6}$$

where $\hat{\eta}_i$ are two-dimensional Pauli matrices $(i = 1, 2, 3)$ or the identity matrix $(i = 0)$ encoding the unit cell degree of freedom.

The generating operators in this case read

$$N_{C_{4z}} = \begin{pmatrix} 0 & 0 & 1 & 0 \\ 0 & 1 & 0 & 0 \\ 1 & 0 & 0 & 0 \\ 0 & 0 & 0 & 1 \end{pmatrix} \otimes \frac{\sigma_0 - i\sigma_3}{\sqrt{2}}, \qquad N_i = \eta_0 \otimes \tau_1 \otimes \sigma_0, \qquad N_{\sigma_d} = \frac{i}{\sqrt{2}} \eta_0 \otimes \tau_0 \otimes (\sigma_1 - \sigma_2),$$

where the $N_{C_{4z}}$ can be decomposed on the basis of Pauli matrices as

$$N_{C_{4z}} = \frac{1}{2}(\eta_0 \otimes \tau_0 - \eta_0 \otimes \tau_3 + \eta_1 \otimes \tau_0 + \eta_1 \otimes \tau_3) \otimes \frac{\sigma_0 - i\sigma_3}{\sqrt{2}}.$$

| (unit cell, sublattice, spin) | $i$ | $\bar{C}_{4z}$ | $\sigma_d$ | $C_{2\bar{d}}$ | $\mathcal{T}$ | irrep |
|---|---|---|---|---|---|---|
| (0,0,0) | + | + | + | + | + | $A_{1g}$ |
| (1,0,0) | + | + | + | + | + | $A_{1g}$ |
| $(0,1,0)+(1,1,0)$ | + | + | + | + | + | $A_{1g}$ |
| (0,0,3) | + | + | − | − | − | $A_{2g}$ |
| (1,0,3) | + | + | − | − | − | $A_{2g}$ |
| $(0,1,3)+(1,1,3)$ | + | + | − | − | − | $A_{2g}$ |
| (0,3,3) | − | + | − | + | − | $A_{1u}$ |
| (1,3,3) | − | + | − | + | − | $A_{1u}$ |
| $(0,2,3)+(1,2,3)$ | − | + | − | + | + | $A_{1u}$ |
| (0,3,0) | − | + | + | − | + | $A_{2u}$ |
| (1,3,0) | − | + | + | − | + | $A_{2u}$ |
| $(0,2,0)+(1,2,0)$ | − | + | + | − | − | $A_{2u}$ |
| $(0,1,3)-(1,1,3)$ | + | − | − | − | − | $B_{1g}$ |
| $(0,1,0)-(1,1,0)$ | + | − | + | + | + | $B_{2g}$ |
| $(0,2,0)-(1,2,0)$ | − | − | + | − | − | $B_{1u}$ |
| $(0,2,3)-(1,2,3)$ | − | − | − | + | + | $B_{2u}$ |
| $\{(0,0,1),(0,0,2)\}$ | $\sigma_0$ | $i\sigma_2$ | $-\sigma_1$ | $\sigma_1$ | − | $E_g$ |
| $\{(1,0,1),(1,0,2)\}$ | $\sigma_0$ | $i\sigma_2$ | $-\sigma_1$ | $\sigma_1$ | − | $E_g$ |
| $\{(0,1,1)+(1,1,1),(1,1,2)+(0,1,2)\}$ | $\sigma_0$ | $i\sigma_2$ | $-\sigma_1$ | $\sigma_1$ | − | $E_g$ |
| $\{(0,1,1)-(1,1,1),(1,1,2)-(0,1,2)\}$ | $\sigma_0$ | $i\sigma_2$ | $\sigma_1$ | $-\sigma_1$ | − | $E_g$ |
| $\{(0,1,1)+(0,1,2),-(1,1,1)+(1,1,2)\}$ | $\sigma_0$ | $i\sigma_2$ | $-\sigma_3$ | $\sigma_3$ | − | $E_g$ |
| $\{(0,1,1)-(0,1,2),(1,1,1)-(1,1,2)\}$ | $\sigma_0$ | $i\sigma_2$ | $\sigma_3$ | $-\sigma_3$ | − | $E_g$ |
| $\{(0,3,1),(0,3,2)\}$ | $-\sigma_0$ | $i\sigma_2$ | $-\sigma_1$ | $-\sigma_1$ | − | $E_u$ |
| $\{(1,3,1),(1,3,2)\}$ | $-\sigma_0$ | $i\sigma_2$ | $-\sigma_1$ | $-\sigma_1$ | − | $E_u$ |
| $\{(0,2,1)+(1,2,1),(1,2,2)+(0,2,2)\}$ | $-\sigma_0$ | $i\sigma_2$ | $-\sigma_1$ | $\sigma_1$ | + | $E_u$ |
| $\{(0,2,1)-(1,2,1),(1,2,2)-(0,2,2)\}$ | $-\sigma_0$ | $i\sigma_2$ | $\sigma_1$ | $-\sigma_1$ | + | $E_u$ |
| $\{(0,2,1)+(0,2,2),-(1,2,1)+(1,2,2)\}$ | $-\sigma_0$ | $i\sigma_2$ | $-\sigma_3$ | $\sigma_3$ | + | $E_u$ |
| $\{(0,2,1)-(0,2,2),(1,2,1)+(1,2,2)\}$ | $-\sigma_0$ | $i\sigma_2$ | $\sigma_3$ | $-\sigma_3$ | + | $E_u$ |

TABLE VI. Classification of order parameter matrices in the enlarged unit cell scenario with definite transformation properties under inversion. A set of indices $(i,j,k)$ corresponds to the matrix $\eta_i\otimes\tau_j\otimes\sigma_k$, as indicated in Eq. 6. Blue and gray correspond to the $M_z$ antiferromagnetic and $P_z$ polar orders, respectively. Note that, as these are homogeneous phases, the irrep labels for these orders match the ones found in the symmetry classification within the single unit cell scenario. The rest of the notation is identical to the one used in Table V.

| (UC,SL,spin) | $i$ | $C_4$ | $\sigma_d$ | $C_{2\bar{d}}$ | $\mathcal{T}$ | irrep |
|---|---|---|---|---|---|---|
| $\{(3,1,0),(2,2,0)\}$ | $\sigma_3$ | $\sigma_1$ | $\sigma_0$ | $\sigma_3$ | + | $E_{1m}$ |
| $\{(2,0,0),(2,3,0)\}$ | $\sigma_3$ | $-\sigma_1$ | $\sigma_0$ | $\sigma_3$ | − | $E_{1m}$ |
| $\{(2,1,0),(3,2,0)\}$ | $\sigma_3$ | $-\sigma_1$ | $\sigma_0$ | $\sigma_3$ | − | $E_{1m}$ |
| $\{(3,0,0),(3,3,0)\}$ | $\sigma_3$ | $-\sigma_1$ | $\sigma_0$ | $\sigma_3$ | + | $E_{1m}$ |
| $\{(3,1,3),(2,2,3)\}$ | $\sigma_3$ | $\sigma_1$ | $-\sigma_0$ | $-\sigma_3$ | − | $E_{2m}$ |
| $\{(2,0,3),(2,3,3)\}$ | $\sigma_3$ | $-\sigma_1$ | $-\sigma_0$ | $-\sigma_3$ | + | $E_{2m}$ |
| $\{(2,1,3),(3,2,3)\}$ | $\sigma_3$ | $-\sigma_1$ | $-\sigma_0$ | $-\sigma_3$ | + | $E_{2m}$ |
| $\{(3,0,3),(3,3,3)\}$ | $\sigma_3$ | $-\sigma_1$ | $-\sigma_0$ | $-\sigma_3$ | − | $E_{2m}$ |
| $\{(202)-(201),(232)+(231)\}$ | $\sigma_3$ | $i\sigma_2$ | $\sigma_3$ | $\sigma_0$ | + | $E_{3m}$ |
| $\{(212)-(211),(322)+(321)\}$ | $\sigma_3$ | $i\sigma_2$ | $\sigma_3$ | $\sigma_0$ | + | $E_{3m}$ |
| $\{(311)-(312),(221)+(222)\}$ | $\sigma_3$ | $i\sigma_2$ | $\sigma_3$ | $\sigma_0$ | − | $E_{3m}$ |
| $\{(302)-(301),(332)+(331)\}$ | $\sigma_3$ | $i\sigma_2$ | $\sigma_3$ | $\sigma_0$ | − | $E_{3m}$ |
| $\{(202)+(201),-(232)+(231)\}$ | $\sigma_3$ | $i\sigma_2$ | $-\sigma_3$ | $-\sigma_0$ | + | $E_{4m}$ |
| $\{(212)+(211),-(322)+(321)\}$ | $\sigma_3$ | $i\sigma_2$ | $-\sigma_3$ | $-\sigma_0$ | + | $E_{4m}$ |
| $\{(311)+(312),-(221)+(222)\}$ | $\sigma_3$ | $i\sigma_2$ | $-\sigma_3$ | $-\sigma_0$ | − | $E_{4m}$ |
| $\{(302)+(301),-(332)+(331)\}$ | $\sigma_3$ | $i\sigma_2$ | $-\sigma_3$ | $-\sigma_0$ | − | $E_{4m}$ |

TABLE VII. Classification of order parameter matrices in the enlarged unit cell scenario without a definite transformation under inversion. Green corresponds to the in-plane magnetic configuration $M_{\text{plane}}$ discussed in the main text. For notation consult Tables V and VI, as well as the main text.

## IV. LANDAU THEORY

Here, we investigate a Landau model containing a primary superconducting order parameter $\Psi$, and a secondary order parameter $\phi$, both taken at first to be single component. The free energy for $\Psi$ and $\phi$ are respectively

$$f_\Psi = a_\Psi|\Psi|^2 + b_\Psi|\Psi|^4,$$
$$f_\phi = a_\phi|\phi|^2 + b_\phi|\phi|^4 \tag{7}$$

where $a_\Psi = \alpha_\Psi(T - T_\Psi)$ and $a_\phi = \alpha_\phi(T - T_\phi)$ with $\alpha_\Psi, \alpha_\phi > 0$. By definition, the critical temperature of the primary order is larger than that of the secondary, $T_\Psi > T_\phi$. Let us now consider possible coupling terms between $\Psi$ and $\phi$. Due to U(1) gauge symmetry, the superconducting order parameter always has to appear in a gauge invariant quadratic form $\Psi^*\Psi$ (or higher powers of it).

One possible coupling is quadratic in both order parameters and reads

$$f_{\lambda_{\rm qq}} = \lambda_{\rm qq}|\phi|^2|\Psi|^2, \tag{8}$$

with $\lambda_{\rm qq}$ a phenomenological coupling constant. In this scenario, the phase diagram features the primary order $\Psi$ setting in at its bare critical temperature $T_\Psi$, which corrects the $|\phi|^2$ term in $f_\phi$, and hence to the critical temperature $T_\phi$. This scenario is shown in Fig. 1(a) in the main text.

Let us now focus on an alternative, linear-quadratic coupling term with coupling constant $\lambda_{\rm lq}$

$$f_{\rm lq} = \lambda_{\rm lq}\phi|\Psi|^2, \tag{9}$$

and assume for the time being that the above term is invariant under all operative symmetries. Below, we show that such coupling term results in the secondary order setting in *simultaneously* with the primary order; see Fig. 1(b) in the main text. Since $T_\Psi > T_\phi$, we first solve for $|\Psi|^2$ as a function of temperature and find

$$|\Psi|^2 = -\frac{\alpha_\Psi}{b_\Psi}. \tag{10}$$

We now minimize the free energy $f = f_\Psi + f_\phi + f_{\rm lq}$ with respect to $\phi$ to find

$$a_\phi(T - T_\phi)\phi + b_\phi\phi^3 = -\frac{\lambda_{\rm lq}a_\Psi}{2b_\Psi}(T_\Psi - T), \tag{11}$$

The linear-cubic equation above is difficult to solve exactly, but one can consider it qualitatively using a geometrical approach. Notice that we are interested in the temperature range $T_\phi < T \le T_\Psi$, where the l.h.s. describes a linear-cubic polynomial with positive coefficients. The corresponding curve is, therefore, monotonically increasing, crossing zero only at $\phi = 0$ as shown in Fig. 1. At $T = T_\Psi$ the r.h.s. vanishes and the only solution is the trivial $\phi = 0$. Conversely, upon lowering the temperature the r.h.s becomes finite, with its sign set by the sign of the coupling $\lambda_{\rm lq}$. In this case Eq. (11) features *no solution* at $m = 0$; rather, it has two solutions at $\phi = \pm|\phi_0|$. The order parameter $\phi$ can change its sign to optimally lower the free energy. This outcome is, therefore, unaffected by the sign of $\lambda_{\rm lq}$.

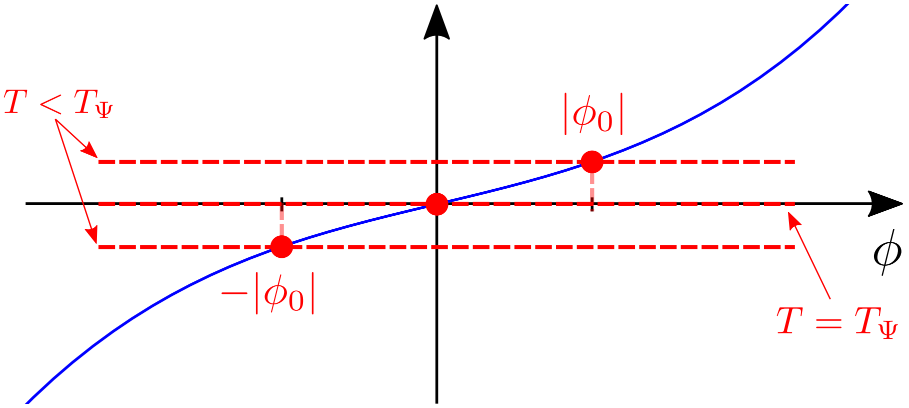


FIG. 1. Geometric solution of Eq. (11). The l.h.s. describes a linear-cubic polynomial in $\phi$ with positive coefficient, yielding a monotonically increasing curve (blue). The r.h.s. (red lines) is constant, and we find a $\phi = 0$ solution when it goes to zero at $T = T_\Psi$. For any $T < T_\Psi$ we find nontrivial solutions $\phi = \pm|\phi_0|$ where the sign of $\phi$ is determined by the sign of the coupling $\lambda_{\rm lq}$.

Notice that while the primary order parameter $\Psi$ sets in with the usual mean-field order parameter critical exponent $\beta = 1/2$, the secondary order parameter $\phi$ develops more gradually, with $\beta = 1$. To see this we focus on the vicinity of $T_\Psi$, where the l.h.s. of Eq (11) is dominated by the linear term, and introduce the reduced temperature $t = \frac{T-T_\Psi}{T_\Psi}$, obtaining

$$\phi = \frac{\lambda_{\rm lq}}{2}\frac{\alpha_\Psi}{\alpha_\phi b_\Psi}\frac{T-T_\Psi}{T-T_\phi} \sim \frac{\frac{T-T_\Psi}{T_\Psi}}{\frac{T-T_\Psi}{T_\Psi}+\frac{T_\Psi-T_\phi}{T_\Psi}} = \frac{t}{t+c} \approx \frac{t}{c}\left(1-\frac{t}{c}\right), \tag{12}$$

where $c = \frac{T_\Psi - T_\phi}{T_\Psi}$ is temperature independent. This corroborates the linear onset of $\phi$ in the leading order.

Let us know consider the case where the secondary order parameter $\phi$ is odd parity. Then, in the linear-quadratic coupling term the superconducting order parameter has to have two-components, $\mathbf{\Psi} = (\Psi_1, \Psi_2)$, with opposite parity. The corresponding free energy term becomes

$$f_\Psi = a_\Psi|\mathbf{\Psi}|^2 + b_{\Psi,1}|\mathbf{\Psi}|^4 + \frac{b_{\Psi,2}}{2}\left[(\Psi_1^*\Psi_2)^2 + (\Psi_1\Psi_2^*)^2\right] + b_{\Psi,3}|\Psi_1|^2|\Psi_2|^2. \tag{13}$$

The stable solutions of $f_\Psi$ describe (a) a nematic superconductor with $\mathbf{\Psi} = (\Psi, 0)$ or $\mathbf{\Psi} = (0, \Psi)$, (b) another nematic superconducting state with $\mathbf{\Psi} = \Psi(1,1)/\sqrt{2}$ or $\mathbf{\Psi} = \Psi(1,-1)/\sqrt{2}$, or (c) a chiral superconductor with $\mathbf{\Psi} = \Psi(1,i)/\sqrt{2}$ or $\mathbf{\Psi} = \Psi(1,-i)/\sqrt{2}$. If $\phi$ describes a time reversal symmetry breaking magnetic order, such as $M_z$ in the main text, the form of the linear-quadratic coupling has to be

$$f_\lambda = i\lambda_{\rm lq}\phi(\Psi_1^*\Psi_2 - \Psi_1\Psi_2^*). \tag{14}$$

In this case, for a nonvanishing coupling term, the superconductor has to be in a chiral phase, $\mathbf{\Psi} = \Psi(1,\pm i)/\sqrt{2}$, where (without loss of generality) we pick the minus sign. The full free energy becomes

$$f_{\rm chiral} = a_\Psi\Psi^2 + b_\Psi\Psi^4 + a_\phi\phi^2 + b_\phi\phi^4 + \lambda_{\rm lq}\phi\Psi^2, \tag{15}$$

with $b_\Psi = b_{\Psi,1} - b_{\Psi,2}/4 + b_{\Psi,3}/4$. The previous analysis can then be applied directly. If, on the other hand, $\phi$ preserves

time reversal symmetry, such as the polar order $P_z$ in the main text, then the form of the coupling becomes

$$f_\lambda = \lambda_{\mathrm{lq}}\phi(\Psi_1^*\Psi_2 + \Psi_1\Psi_2^*). \tag{16}$$

For this to be nonvanishing, the superconducting order parameter has to be nematic $\mathbf{\Psi} = \Psi(1,1)/\sqrt{2}$ (where we choose the positive sign). The full free energy is of a similar form, reading

$$f_{\mathrm{nematic}} = a_\Psi\Psi^2 + b_\Psi\Psi^4 + a_\phi\phi^2 + b_\phi\phi^4 + \lambda_{\mathrm{lq}}\phi\Psi^2, \tag{17}$$

with $b_\Psi = b_{\Psi,1} + b_{\Psi,2}/4 + b_{\Psi,3}/4$.

---

[1] C. Bradley and A. Cracknell, *The Mathematical Theory of Symmetry in Solids: Representation Theory for Point Groups and Space Groups*, EBSCO ebook academic collection (OUP Oxford, 2010).
